# Supplementary material for: Data-Driven Design Rules for TADF Emitters from a High-Throughput Screening of 747 Molecules
Source: arXiv:2511.11606 source file (2026-03-19)
Supplement: Supplementary file 1 [file SI_Table_Validation_379mol_preview.tex]

\begin{table}[H]
\centering
\caption{Experimental validation dataset (379 molecules). Full table available in CSV format.}
\label{tab:validation_massive}
\small
\begin{tabular}{llcccccc}
\hline
Molecule & Arch. & Exp & Calc$_{\text{Gas}}$ & Calc$_{\text{Tol}}$ & Error & $f$ & DOI \\
\hline
Diphenylsulfane & 0D-1A & 0.280 & 0.094 & -0.002 & -0.186 & 0.001 & \cite{10.1039/D2TC01435A} \\
CzmPPC & 0D-1A & 0.280 & 0.103 & 0.074 & -0.177 & 0.001 & \cite{10.1039/D2TC01435A} \\
TCbTrz & 0D-1A & 0.270 & 0.220 & 0.315 & -0.050 & 0.381 & \cite{10.1039/C8NJ00767E} \\
APPT & 0D-1A & 0.070 & 0.186 & 0.229 & +0.116 & 0.011 & \cite{10.1016/j.dyepig.202...} \\
PX-TRZ & 0D-1A & 0.056 & 0.242 & 0.253 & +0.186 & 0.031 & \cite{10.1039/C9TC06497D} \\
DMIC-TRZ & 0D-1A & 0.056 & 0.519 & 0.755 & +0.463 & 0.231 & \cite{10.1016/j.orgel.2022...} \\
D–A–D & 0D-2A & 0.242 & 0.028 & 0.011 & -0.214 & 0.007 & \cite{10.1039/D1TC05730H} \\
phenazasiline & 0D-2A & 0.242 & 0.028 & 0.011 & -0.214 & 0.007 & \cite{10.1039/D1TC05730H} \\
TPA-CN-N4 & 0D-2A & 0.190 & 0.024 & 0.036 & -0.166 & 0.007 & \cite{10.1039/D1MH01651B} \\
DTRZSFX & 0D-2A & 0.310 & 0.356 & 0.375 & +0.046 & 2.021 & \cite{10.1016/j.dyepig.202...} \\
mTPA–PPI & 1D-0A & 0.760 & 0.258 & 0.270 & -0.502 & 0.535 & \cite{10.1039/C5SC01131K} \\
mTPA-PPI & 1D-0A & 0.760 & 0.260 & 0.272 & -0.500 & 0.556 & \cite{10.1039/C5SC01131K} \\
DPACPhTPI & 1D-0A & 0.720 & 0.255 & 0.250 & -0.465 & 0.472 & \cite{10.1016/j.dyepig.201...} \\
PTPC & 1D-0A & 0.636 & 0.244 & 0.229 & -0.391 & 0.473 & \cite{10.1039/D2QM00506A} \\
mP2MPC & 1D-0A & 0.650 & 0.284 & 0.298 & -0.366 & 0.306 & \cite{10.1016/j.cej.2022.1...} \\
9PhCzFDBFSPO & 1D-0A & 0.690 & 0.352 & 0.379 & -0.338 & 0.218 & \cite{10.1016/j.cej.2019.1...} \\
9PhCzFDBFDPO & 1D-0A & 0.630 & 0.354 & 0.377 & -0.276 & 0.207 & \cite{10.1016/j.cej.2019.1...} \\
BFDMAc-NAI & 1D-0A & 0.235 & 0.104 & 0.128 & -0.131 & 0.091 & \cite{10.1039/C9TC01973A} \\
TX-CzPh & 1D-0A & 0.670 & 0.551 & 0.552 & -0.119 & 0.170 & \cite{10.1039/D1TC02324A} \\
PXZ-PPO & 1D-0A & 0.600 & 0.510 & 0.538 & -0.090 & 0.610 & \cite{10.1039/D0TC03747H} \\
\multicolumn{8}{c}{... (359 more molecules in CSV file) ...} \\
\hline
\end{tabular}
\end{table}
